# Supplementary material for: Identification and minimization of losses in microscaled spin-wave transducers
Source: arXiv:2505.08656 source file (2025-05-19)
Supplement: Supplementary file 1 [file Supplementary_information_-_Identification_and_minimization_of_losses_in_microscaled_spin-wave_transducers.pdf]

# Supplementary information - Identification and minimization of losses in microscaled spin-wave transducers

Felix Kohl,<sup>1,\*</sup> Björn Heinz,<sup>1</sup> Ádám Papp,<sup>2,3</sup> Györgi Csaba,<sup>2,3</sup> and Philipp Pirro<sup>1</sup>

<sup>1</sup>*Fachbereich Physik and Landesforschungszentrum OPTIMAS,  
Rheinland-Pfälzische Technische Universität Kaiserslautern-Landau, D-67663 Kaiserslautern, Germany*

<sup>2</sup>*Faculty of Information Technology and Bionics,  
Pazmany Peter Catholic University, Budapest, Hungary*

<sup>3</sup>*Jedlik Innovation Kft., Budapest, Hungary*

## CONTENTS

|                                                        |   |
|--------------------------------------------------------|---|
| I. Spin-wave dispersion relation and avoided crossings | 1 |
| II. Impact of group velocity on transmission spectra   | 3 |
| III. Numerical calculation of spin-wave impedances     | 4 |
| IV. Spin-wave decay length                             | 6 |
| V. Comparison of coplanar waveguide antennas           | 7 |
| References                                             | 8 |

## I. SPIN-WAVE DISPERSION RELATION AND AVOIDED CROSSINGS

In the main text, spin-wave transmission is compared for the same structure across different YIG thicknesses. To illustrate this more clearly, Fig. S1 presents the dispersion relations for the YIG films, calculated by TetraX [1, 2], used in the Damon-Eshbach geometry, alongside the wave-vector distribution of the antenna field. The slope of the dispersion curve represents the group velocity, which determines the spin-wave propagation speed at a given wave vector or frequency. The antennas are specifically designed to primarily excite spin waves in regions of high group velocity across all YIG films, minimizing propagation losses associated with slow spin waves.

Comparing the slope of thin and thick YIG film spin-wave dispersions, it is apparent that thicker YIG films exhibit higher group velocities, which, assuming constant Gilbert damping, leads to lower propagation losses. Notably, for thicker YIG films, the flattening of the dispersion curve, leads to decreasing group velocity at higher wave-vectors. This means that while damping-related losses remain low at small wave vectors, they increase significantly at larger wave vectors. Consequently, in the measured transmission spectra, the second and third excitation maxima of the antenna are increasingly suppressed for higher wave vectors. A similar impact of changing group velocity is presented in Section II.

As the YIG thickness increases, the exchange energy of higher quantized modes (perpendicular standing spin waves, PSSW) decreases. As a result, the frequencies of these modes are closer to those of the fundamental mode. From a thickness of 209 nm on, they are so low in their frequencies that they intersect the fundamental mode in the steep, dipolar-dominated region of the fundamental mode. At the intersection points, both modes hybridize with each other and form a narrow frequency gap, which is referred to as an avoided crossing. With increasing thickness, the number of these gaps within the operating band of the transducer increases, e.g., as is the case for the 799 nm thick YIG. Since the group velocity decreases sharply near these gaps or even no spin waves can be excited at all in the gap, dips in the transmission spectrum are to be expected at these points.

The finite element solver TetraX [2] enables the calculation of both the eigenvalues (dispersion relation) and the eigenvectors (mode profiles along the layer thickness) of the investigated magnetic systems. This is illustrated using the thickest YIG film from the experiments, as it shows the most mode crossings. Figure S2 shows the calculated dispersions alongside a color plot of the mode profiles, indicating the local amplitude of the dynamic magnetization

---

\* [fkohl@rptu.de](mailto:fkohl@rptu.de)

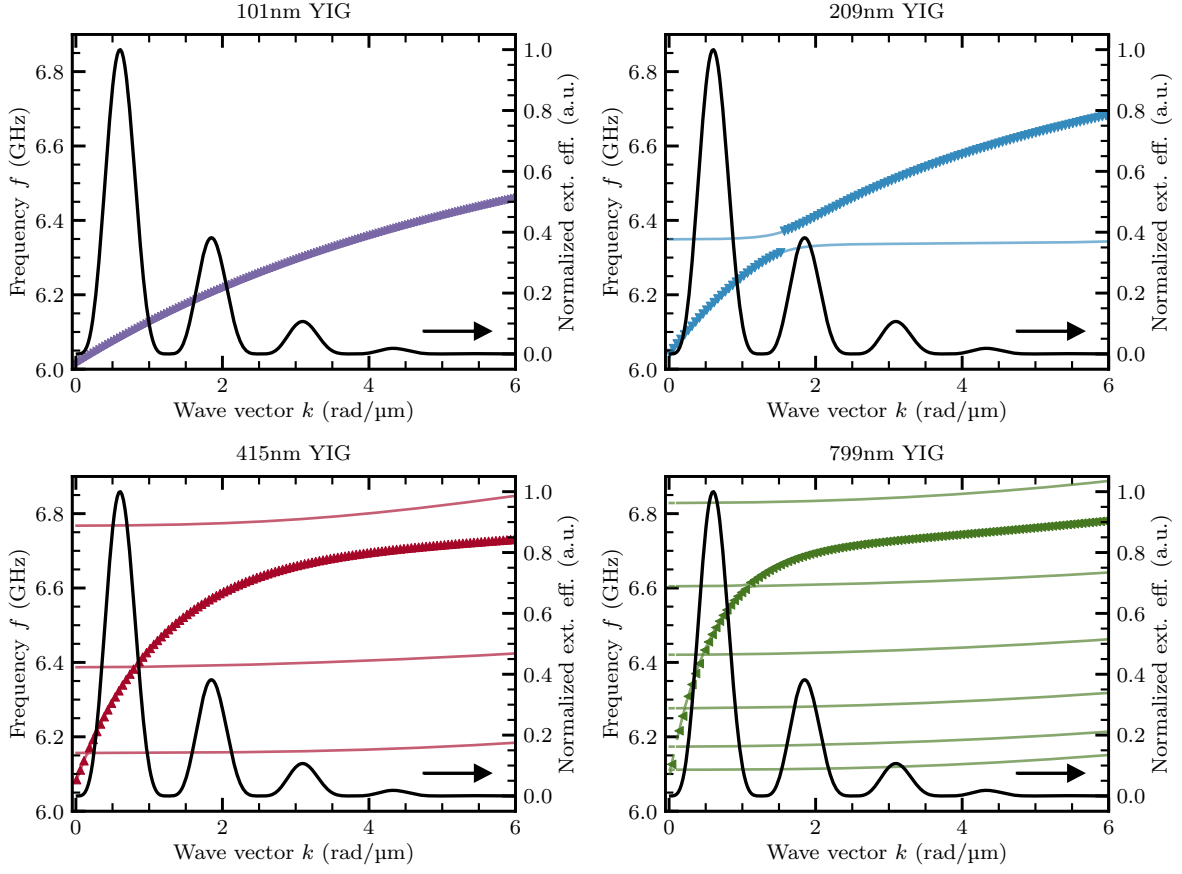

FIG. S1. Calculated spin-wave dispersion relations in Damon-Eshbach geometry for YIG films of different thicknesses. Calculations are performed for an external field of  $\mu_0 H_{\text{ext}} = 139$  mT. The fundamental mode is plotted by markers, higher quantized modes are represented in thin lines. The normalized antenna field wave-vector spectrum is shown in black.

along the layer thickness. The extracted mode of interest is highlighted in white, while all others are shown in red. For the fundamental surface mode (Damon-Eshbach mode (DE)), an exponential decay of the dynamic magnetization along the film thickness is expected, scaling with  $k \cdot t$ . Given the small wave vectors and thicknesses considered here, the profile of this mode remains nearly homogeneous. In contrast, higher-order thickness modes exhibit multiple nodal points due to quantization effects.

In S2 a) the mode profile is shown according to the DE mode. The profile of this mode along the thickness remains largely homogeneous and is only distorted for wave vectors close to the avoided crossings with a higher quantized mode. This indicates that the fundamental mode character is effectively passed on across avoided gaps, and only at these hybridization points does the mode profile experience significant deformation before transitioning into the next higher-order mode. Therefore, in the experiment, the spin-wave excitation should not be influenced for frequencies in between these avoided crossings. The distortions of the profile occurring towards higher wave vectors in the figure are a consequence of the extremely broad avoided crossings with the highest PSSW mode shown. In the right part of the figure, the course of a higher quantized mode is followed as an example. Here, too, it is clear that this shows a profile with several nodes before the crossing, followed by a homogeneous profile. At the subsequent crossing with the next higher PSSW mode, the mode then inherits the profile of this mode and passes on the homogeneous profile of the fundamental mode.

To illustrate the influence of the mode crossings, a spectrum measured on the 799 nm thick YIG film is shown in Fig. S3 along with the calculated dispersion relation. Within the main maximum in the transmission spectrum, a narrow dip in transmission can be seen. In comparison with the dispersion relation, it can be seen that the position of this dip is close to the frequency of a crossing of two modes. The deviation is attributed to possible inaccuracies in the field measurement and film parameters. Please note, variation of the magnetic field may introduce a relative shift of mode crossing and maximum transmission point, eventually pushing it out of the transmission band.

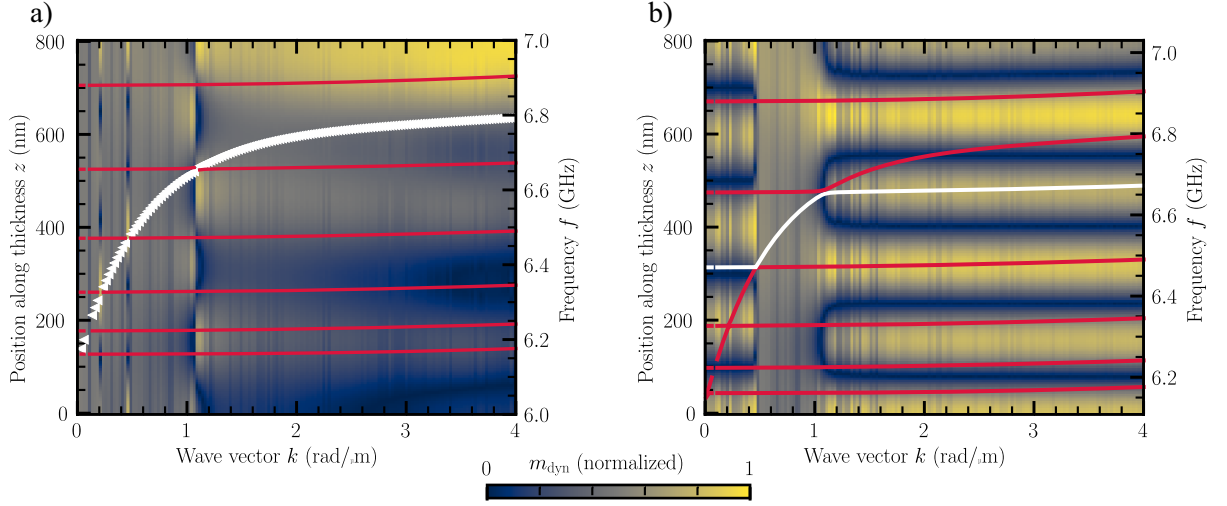

FIG. S2. Calculated dispersion relation for a 799 nm thick YIG film. Coded in color is the normalized magnitude of the dynamic magnetization of the fundamental mode in a) (shown in white) and one exemplary mode in b) as function of wave-vector and position along the film thickness. Parameters for the calculation are  $\mu_0 H_{\text{ext}} = 140$  mT,  $M_s = 159.8$  kA m $^{-1}$  and  $A_{\text{ex}} = 3.5$  pJ/m $^3$ .

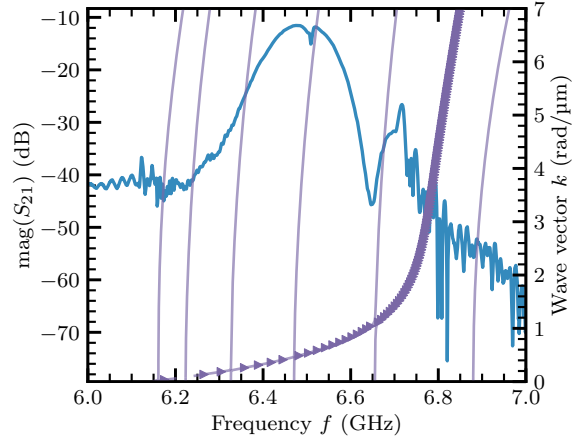

FIG. S3. Measured transmission spectrum for the 799 nm thick YIG at an external field of 140 mT. In purple the calculated dispersion relation using the parameter  $M_s = 159.8$  kA m $^{-1}$  and  $A_{\text{ex}} = 3.5$  pJ/m $^3$  is shown.

## II. IMPACT OF GROUP VELOCITY ON TRANSMISSION SPECTRA

In the main text of the paper, tunability of the operational frequency via the external magnetic field is investigated. According to the model [3] quoted in the main text, the shape of the transmission spectra depends strongly on the excitation efficiency of the antennas but also on the dispersion. All measurements carried out for this work are performed in the Damon-Eshbach geometry. For these, an increase in the external magnetic field leads to a flatter dispersion relation and thus also to a lower group velocity. Analogous to the exemplary observation of the spectra in the main text, calculations for the 209 nm thick YIG film are shown here again. The calculated dispersions using TetraX [1, 2] are shown in Fig. S4 a) and b) for field strengths of 140 mT and 450 mT together with the group velocities derived from them. For the calculation,  $M_s = 155.3$  kA m $^{-1}$  and  $A_{\text{ex}} = 3.5$  pJ/m $^3$  were used. The calculations clearly show the avoided crossings if DE mode and the first standing spin wave mode were to cross. A direct comparison of the two field strengths clearly shows the flatter dispersion and correspondingly lower group velocity of the DE mode. Transferred to the excitation efficiency of the antennas in wave vector space, this means that for high field strengths the same  $k$ -interval is mapped to a smaller frequency interval in the recorded spectra. Accordingly, it is expected that with increasing field strengths in the experiment, the individual peaks of the antenna efficiencies become narrower and move closer together. At the same time, the influence of spin wave attenuation also increases, as the spin waves

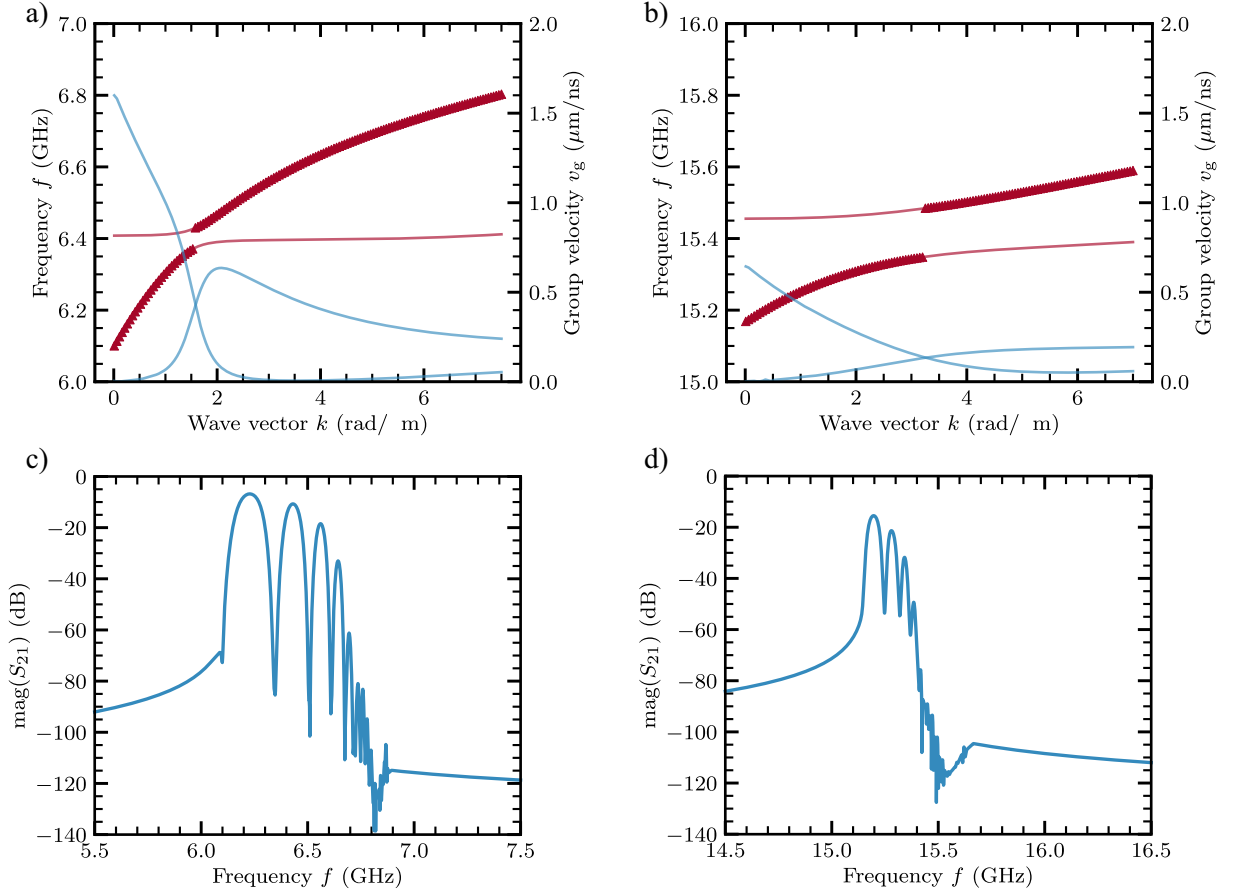

FIG. S4. a), b): Calculated dispersion relations and group velocities of the two lowest modes for a 209 nm thick YIG film and external field values of 140 mT and 450 mT. c), d) Calculated transmission spectra neglecting antenna properties using the simple analytic approximation from [3].

propagate slower. An exemplary calculation of the transmission spectra for the considered cases is shown in Figure S4.c) and d) using the analytical model from [3] and neglecting the electrical antenna properties. It clearly shows the narrower shape of the spectrum with closer but also weaker peaks. The weaker drop in amplitude in the minima can be explained by the line width of the individual excitations, which project further into the minima due to the narrower shape of the spectrum.

### III. NUMERICAL CALCULATION OF SPIN-WAVE IMPEDANCES

Simulations were carried out with the model from [4] to determine the real spin wave resistances and the electrical resistances of the antennas for a 799 nm thick YIG film at an external field of 135 mT. The parameters for the YIG are the same as used before. Due to the large thickness of the YIG, the grid for the micromagnetic simulations is discretized in 20 layers to include the inhomogeneous magnetization profile of the PSSW modes. The spin-wave induced Z-Parameters obtained from the simulation are shown in Fig. S5. Within these traces, two maxima can be found. By comparing to the previously considered antenna excitation efficiency and the spin-wave dispersion relation in Fig. S1 d), the first maximum can be interpreted as the main excitation maximum of the antenna, while the second narrower peak is attributed to the second and third maximum of the antenna excitation efficiency. These are larger in the self-impedance as the main peak, as the group velocity at these frequencies is strongly decreased. Consequently a larger interval of wave-vectors contributes to these impedances as for the main peak, in the steeper region of dispersion relation. As low group velocity is connected to larger losses during spin-wave propagation, the second and third peak in the mutual impedance are significantly lower than the one of the main peak. This matches the observation in the experiment, that the signal transmission from the main peak is significantly stronger than the second and third antenna maxima.

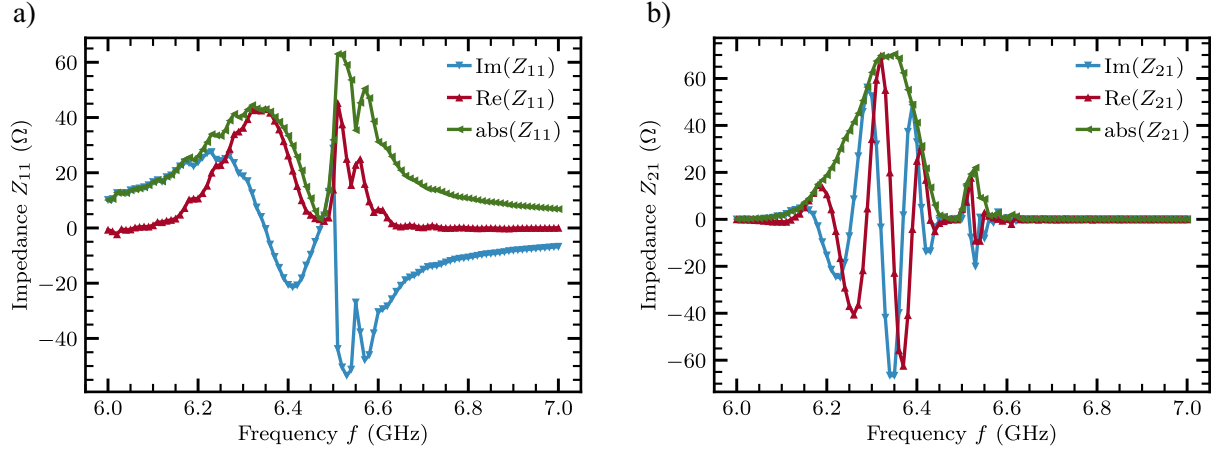

FIG. S5. Self (a) and mutual (b) spin-wave impedances obtained from the simulations of a 799 nm thick YIG film at an external field of 135 mT.

The same type of numerical calculation is performed for the same magnetic system but the thickness of the antenna metal lines is increased up to 900 nm. For each simulation the maximum value of the first maximum in the real part of the self-impedance  $R_{\text{sw}} = \text{Re}(Z_{11})$  is extracted along with the magnitude of the electric resistance obtained from electromagnetic simulations, as outlined in [4]. The results are presented in Fig. S6 a). Both, the spin-wave induced resistance as well as the electric resistance decrease for increasing antenna thickness. For the electric resistance, this can intuitively be understood by the increasing diameter of the current carrying lines, reducing the current density and therefore the electric resistance. Decreasing current density is directly related to lower rf magnetic fields generated by the antennas, which in turn decreases the spin-wave inductance, as can be seen from the model in [3], presented in the main text. In other words, as the antenna thickness increases, a greater proportion of the electric current flows further away from the magnetic YIG film and therefore the overlap between the spin wave mode profiles and the dynamic magnetic fields of the antennas decreases. This then leads to a lower spin wave induced impedance. An analogous argumentation for forward volume spin waves is explained in [5].

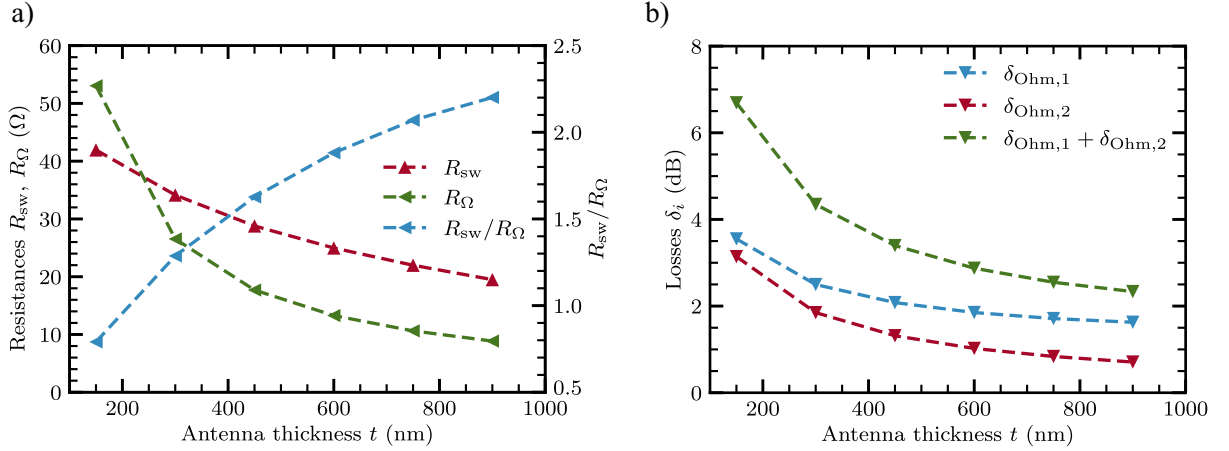

FIG. S6. a) Electrical resistance and maximum spin-wave resistance obtained from numerical calculations. The ratio of spin-wave to electrical resistance is a measure for the ratio of power transferred to the spin-wave system relative to Joule heat. b) Ohmic loss contributions, defined in the main text, as function of antenna thickness.

Overall, however, the electrical resistance in the thickness range under consideration decreases stronger than the spin wave resistance. The ratio of both resistances is proportional to the ratio of the power transferred into the spin wave system relative to the proportion of power converted in the form of Joule heat. The ratio is also shown in Fig. S6 a). Here it can already be seen that, coming from thin antennas, it is beneficial to increase antenna thickness, to increase efficiency. Following the definition of the ohmic loss contributions in the main text, the relative loss contributions can be calculated as function of antenna thickness. The results are presented in Fig. S6 b). From

these results it can be directly concluded that the ohmic losses, which were identified as the largest loss channel in the main text, can be significantly reduced by increasing the antenna thickness. According to the estimate shown, a reduction in losses of more than 4 dB would be possible. At the same time, however, it is also clear that a simple increase in antenna thickness is not possible and useful indefinitely, as the reduction in losses saturates and hardly any improvements can be achieved at very high thicknesses.

#### IV. SPIN-WAVE DECAY LENGTH

For the determination of the spin wave decay length in the experiment, the signal transmission is measured on several structures on the 799 nm thick YIG film with increasing distance between the antennas. The smallest edge-to-edge distance is 10  $\mu\text{m}$ , the largest is 500  $\mu\text{m}$  to show a clear exponential drop in the transmission amplitude. The transmission is measured for all these structures at different magnetic fields. Then, the maximum signal transmission of each structure and external field value is plotted as a function of the antenna distance and an exponential drop in amplitude is assumed. By forming the logarithm of the amplitude, a linear regression can then be performed to determine the spin wave decay length, as parameter  $\lambda_{\text{decay}}$ . To do this, the adapted expression for the signal transmission

$$\log(|S_{21}|) = -\frac{x}{\lambda_{\text{decay}}} + y_0 \quad (\text{S1})$$

with the parameter  $y_0$  for the initial amplitude and the spin-wave decay length  $\lambda_{\text{decay}}$ . The resulting linear fit as well as the measured maximum transmission amplitudes are shown in the inset of Fig. S7 a) for an exemplary field of 139 mT.

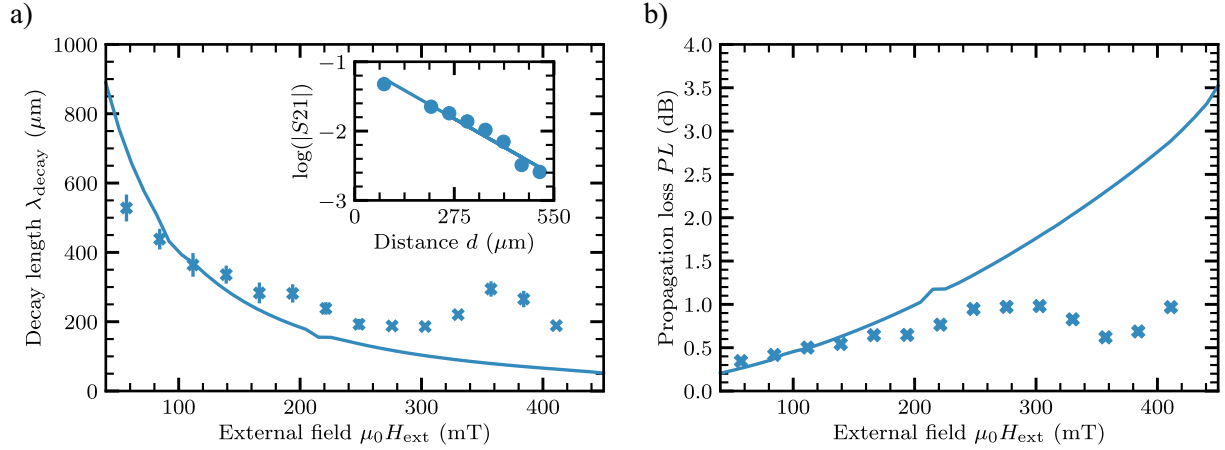

FIG. S7. a) Measured and calculated decay length as function of the external field for 799 nm thick YIG. The inset shows an exemplary fit to determine the decay length at an external field of 139 mT. b) Calculated and measured propagation loss as function of external field using the decay length from a).

The lowest field value of 30 mT was excluded in the evaluation, as it was not possible to determine the decay length from the experimental data without diverging inaccuracies. In addition to the measured decay lengths, a numerical calculation of the decay lengths is shown. This was calculated using TetraX to determine the decay length according to:

$$\lambda_{\text{decay}} = v_g \cdot \tau \quad (\text{S2})$$

with the group velocity  $v_g$  obtained as gradient of the numerically calculated dispersion relation  $\omega(k)$  and the spin-wave lifetime according to [6]

$$\tau^{-1} = \alpha \omega \frac{\partial \omega}{\partial \omega_H}. \quad (\text{S3})$$

Here  $\omega_H = \gamma\mu_0 H_{\text{ext}}$  and the derivative with respect to  $\omega_H$  is calculated numerically by evaluating the dispersion relation for the same  $k$  but  $H_{\text{ext}}$  shifted by a small increment up and down. For the calculation  $\alpha = 2 \cdot 10^{-4}$  is assumed. The agreement with the experimental data is reasonably good. However, the increase at high field values cannot be remodelled as it can probably be attributed to the weak signal amplitudes for these points. Additionally this determination of the decay length has to be interpreted as an upper limit as it neglects any effect of diffraction especially for the larger distances. Nevertheless it can be used to estimate the losses due to spin-wave damping in the devices. Especially at lower fields decay length are significantly larger than the spacing for the structures of the main text. Consequently the energy losses are small. Using the expression for the losses due to spin-wave propagation in the main text, a conversion of decay length to the loss contribution is possible. The values obtained from the experiment as well as numerical calculations are presented in S7.b). Across the whole field range, experimentally determined loss contributions remain smaller than 1 dB, indicating, that the contribution of spin-wave damping in the present spin-wave transducers is not the main contribution limiting efficient operation. The calculated values, however, are significantly larger towards higher fields, and therefore small decay length. This indicates, that for efficient design, low-damping is crucial and propagation distance should be as small as possible.

## V. COMPARISON OF COPLANAR WAVEGUIDE ANTENNAS

In order to test the influence of a reduction in the ohmic resistance of the antennas used on the spin wave transmission, additional structures made of aluminum with two different thicknesses of 150 nm and 400 nm on 799 nm thick YIG are produced. The DC resistance of both structures is measured using a sourcemeter. These results in resistances of  $R_{150\text{ nm}} = 60.7\ \Omega$  and  $R_{400\text{ nm}} = 35.7\ \Omega$ . By increasing the antenna thickness, a significant reduction in resistance is achieved while maintaining the same wave vector spectrum of the antenna field. Based on the division of the loss channels in the main text, an increase in spin wave transmission of approximately 2.1 dB is therefore expected for the thicker structure, which is shown in the points of maximum spin wave transmission for the entire tested field range. However, since the wave vector spectrum of the antenna is the same for both thicknesses, this increase in spin wave transmission is not only expected at the point of maximum transmission, but across the entire band. For comparison, two exemplary spectra of both antennas are shown in Fig. S8 a). The shape of the spectra is identical except for a small frequency offset, which is due to a deviation of the external field by 2 mT. Oscillations can be seen below the main maximum, which can be attributed to the influence of the taper lines. This is followed by a strong main maximum, followed by a weaker second maximum and subsequent rapid oscillations due to the interaction of the higher maxima with the electrical crosstalk. In the middle of the main maximum, a dip can be seen in both spectra, which is explained by a hybridization gap due to a PSSW. Over the entire main maximum, the transmission of the thick antenna is stronger than that of the thin antenna. From this it can be concluded that an overall improvement in transmission can be achieved across the entire band by reducing the ohmic resistance.

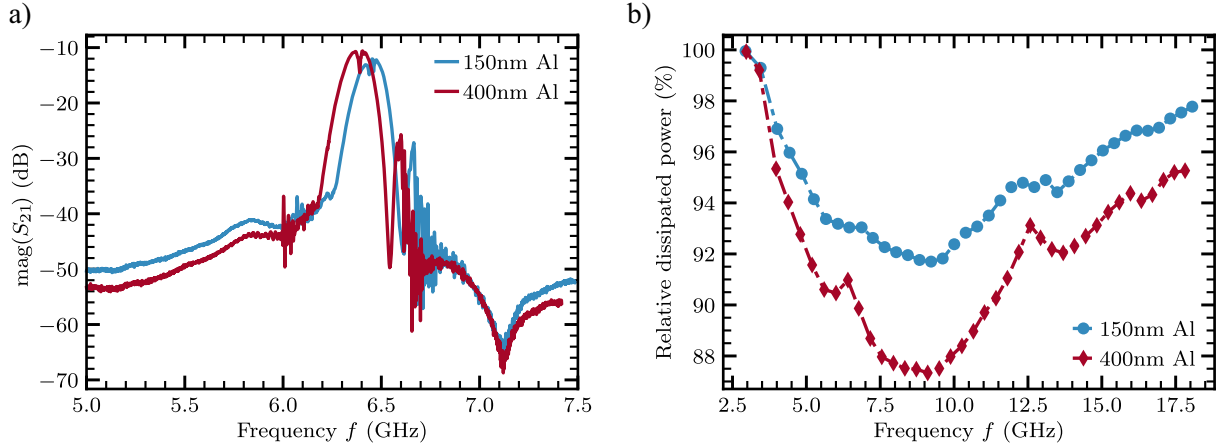

FIG. S8. a) Comparison of spin-wave transmission spectra for an external field of 139 mT. b) Relative fraction of dissipated power relative to the power that is inserted into the device.

After it has been shown that a reduction of the ohmic resistance leads to an increase in transmission, it should now also be evaluated whether this also leads to reduced losses. By reducing the ohmic resistance, the total impedance of the thick CPW is lower than that of the thin CPW. Therefore, lower reflections are measured at the point of maximum

spin wave transmission for the thick antennas. Therefore, in the direct decomposition of reflected, transmitted and dissipated powers as in the main text of the paper, the thicker the antennas appear to increase the transmission only by reducing the reflections, while the amount of dissipated power remains the same. However, this consideration ignores the fact that in the case of thick antennas, a relatively larger proportion of the total power actually reaches the antennas, while a constant proportion of the total power is dissipated. At this point, it therefore makes more sense to compare the proportion of dissipated power relative to the power actually fed into both antennas in order to remove the influence of the reduced reflections. Therefore, in Fig. S8 b), the proportion of dissipated power relative to the power actually inserted is plotted according to

$$\epsilon_{\text{diss|inserted}} = \frac{P_{\text{diss}}}{P_{\text{inserted}}} = \frac{(1 - |S_{21}|^2 - |S_{11}|^2)}{(1 - |S_{11}|^2)} \cdot 100\% \quad (\text{S4})$$

This direct comparison clearly shows that the improved transmission is not only due to lower reflections but also to lower dissipation in the structures themselves. Therefore, reducing the losses by adjusting the thickness of the antennas is a valid way to improve the efficiency of the structures and can help to address several sources of inefficiency, namely strong reflections and ohmic losses, simultaneously.

- 
- [1] L. Körber, G. Quasebarth, A. Otto, and A. Kákay, [AIP Advances](#) **11**, 095006 (2021).
  - [2] L. Körber, G. Quasebarth, A. Hempel, F. Zahn, A. Otto, E. Westphal, R. Hertel, and A. Kákay, “[TetraX: Finite-Element Micromagnetic-Modeling Package](#),” (2022).
  - [3] F. Vanderveken, V. Tyberkevych, G. Talmelli, B. Sorée, F. Ciubotaru, and C. Adelmann, *Scientific Reports* **12**, 3796 (2022).
  - [4] R. Erdélyi, G. Csaba, L. Maucha, F. Kohl, B. Heinz, J. Greil, M. Becherer, P. Pirro, and Á. Papp, *Scientific Reports* **15**, 9806 (2025).
  - [5] M. Robbins, D. Connelly, and J. Chisum, [IEEE Microwave and Wireless Components Letters](#) **32**, 684 (2022).
  - [6] A. Prabhakar and D. D. Stancil, *Spin waves: Theory and applications*, Vol. 5 (Springer, 2009).
